# Supplementary material for: Generative Design of Functional Metal Complexes Utilizing the Internal Knowledge of Large Language Models
Source: arXiv:2410.18136 source file (2024-10-21)
Supplement: Supplementary file 1 [file 09_appendix.tex]

\appendix

\title{\textit{Supplementary Information} for "Optimal Transport for Generating Transition State in Chemical Reactions"}

\maketitle

\renewcommand{\thetable}{\arabic{table}}  
\renewcommand{\thefigure}{\arabic{figure}}
\setcounter{figure}{0}
\setcounter{table}{0}

\makeatletter
\renewcommand{\fnum@figure}{\textbf{Figure \thefigure}. }
\renewcommand{\fnum@table}{\textbf{Table \thetable. }}

% \renewcommand*\contentsname{Table of Contents}
% \tableofcontents
% \listoftables
% \listoffigures

\addcontentsline{toc}{section}{Abbreviation}
\section*{Abbreviation}
The following is the list of abbreviation utilized in the main paper.
\begin{enumerate}
    \item React-OT: \underline{O}ptimal \underline{t}ransport for elementary \underline{react}ions
    \item OA-ReactDiff: \underline{O}bject-\underline{a}ware SE(3) GNN for generating sets of 3D molecules in elementary \underline{react}ions under the \underline{diff}usion model
    \item RMSD: Root mean square deviation.
    \item SE(3): Special Euclidean group in 3D space.
    \item TS: Transition state.
    \item MAE: Mean absolute error.
\end{enumerate}

\section{Physical symmetries and constraints in an elementary reaction.}
\label{Supp:required_symmetries}
An elementary reaction that consists of $n$ fragments as reactant and $m$ fragments as product can be described as $\{\mathrm{R}^{(1)}, ..., \mathrm{R}^{(n)}, \mathrm{TS}, \mathrm{P^{(1)}}, ...,  \mathrm{P^{(m)}}\}$. This reaction requires the following symmetries:
\begin{enumerate}
    \item \textit{Permutation symmetry among atoms in a fragment}. For any fragment in $\mathrm{R}^{(i)}, \mathrm{TS}, \mathrm{P^{(j)}}$, change of atom ordering preserves the reaction.
    \item \textit{Permutation symmetry among fragments in reactant and product}. The change of ordering in $\{\mathrm{R}^{(1)}, ..., \mathrm{R}^{(n)} \}$ and $\{\mathrm{P}^{(1)}, ..., \mathrm{P}^{(m)} \}$ preserve the reaction.
    \item \textit{Rotation and translation symmetry for each fragment}. Rotation and translation operations on any fragment (i.e., $\mathrm{R}^{(i)}, \mathrm{TS}, \mathrm{P^{(j)}}$) preserve the reaction.
\end{enumerate}

\section{Reaction network exploration with React-OT.}
\label{Supp:reaction_network}
To demonstrate the practical application of React-OT in reaction network exploration, the reaction network of $\gamma$-ketohydroperoxide (KHP), a well-studied system commonly used as a benchmark in recent studies.\cite{grambow2018KHP,naz2020unimolecular,QiyuanNCS2021,zhao2022YARP2} Building on reactions generated via graph-based enumeration,\cite{QiyuanNCS2021} we utilized React-OT to determine transition states, which are then used to evaluate activation energies at $\omega$B97X/6-31G* level of theory. A two-step reaction network was constructed based on the predicted activation energies and compared with the network generated by the Yet Another Reaction Program (YARP).\cite{zhao2022YARP2} To manage network size and emphasize kinetically significant reactions, a straightforward growth rule was applied: each node expansion permits the generation of up to five branches, prioritizing reactions with the lowest energy barriers. 

The resulting network generated by React-OT has identical nodes as the one generated by YARP (note: reactant and transition state energies are evaluated at $\omega$B97X/6-31G*, and B3LYP-D3/TZVP//$\omega$B97X/6-31G* level of theory, respectively), indicating that all key reactions were captured, with a mean absolute energy difference of 3.84 kcal/mol (Fig. \ref{Supp:KHPNET}). This case study illustrates how React-OT can be applied to speed up the reaction network exploration.

\begin{figure*}[t!]
    % \centering
    \includegraphics[width=0.7\textwidth]{SI/SA-KHP.pdf}
    % \vspace{-5 pt}
    \caption{\textbf{Reaction Network of $\gamma$-ketohydroperoxide (KHP)}. A two-step reaction network of KHP generated by the Yet Another Reaction Program. Numbers denoted by red/black refer to activation energies computed on DFT-optimized/React-OT-generated transition states.}
    \label{Supp:KHPNET}
    % \vspace{-10 pt}
\end{figure*}

\begin{figure*}[htbp]
    \includegraphics[width=0.58\textwidth]{SI/S1_rmsd_guess.pdf}
    \caption{\textbf{RMSD between the true TS different initial guesses.} 
    Linear interpolation between reactants and products (blue) and samples from a Gaussian distribution (red).
    }
    \label{Supp:rmsd_guss}
\end{figure*}

\begin{figure*}[t!]
    \includegraphics[width=0.68\textwidth]{SI/S2.pdf}
    \caption{\textbf{Additional performance comparison between React-OT and OA-ReactDiff.}
    Cumulative probability for RMSD (top) and barrier height (bottom) for React-OT (red) and OA-ReactDiff + best sample in 40 runs (blue) both shown in log scale for visibility.
    Note that the performance of OA-ReactDiff + best sample in 40 runs is not practically achievable as one does not know the best sample a priori.
    }
    \label{Supp:ot_vs_diff_best}
\end{figure*}

\begin{figure*}[t!]
    \includegraphics[width=0.6\textwidth]{SI/S3_nfe_time.pdf}
    \caption{\textbf{Sampling cost at different number of function evaluation.}
    }
    \label{Supp:nfe_vs_time}
\end{figure*}

\begin{figure*}[t!]
    \includegraphics[width=0.55\textwidth]{SI/S4_points_barrier_error.pdf}
    \caption{\textbf{Persistent barrier height errors.}
    Box plots with all points shown for barrier height errors obtained by React-OT with RGD1-xTB pretraining and training from scratch. 
    The barrier height is shown in log scale with a trucation of 0.5 kcal/mol.
    }
    \label{Supp:persistent_high_error}
\end{figure*}

\begin{figure*}[t!]
    \includegraphics[width=0.5\textwidth]{SI/S6_non_octect_examples.pdf}
    \caption{\textbf{Examples of TS structures breaking the octet rule that React-OT gives large errors.}
    Atoms colored as follows: gray for C, blue for N, red for O, and white for H.
    }
    \label{Supp:non_octect_examples}
\end{figure*}

\begin{figure*}[t!]
    \includegraphics[width=0.5\textwidth]{SI/S5.pdf}
    \caption{\textbf{RMSD between xTB and DFT optimized reactants and products.}
    Distribution of RMSD for reactants (top) and products (bottom) grouped by the reaction type: uni-molecular reaction in blue and multi-molecular reaction in red.
    }
    \label{Supp:xtb_rmsd}
\end{figure*}

\begin{figure*}[t!]
    \includegraphics[width=0.55\textwidth]{SI/S8.pdf}
    \caption{\textbf{Summary of performance for React-OT and OA-ReactDiff}.
    Barrier height, RMSD (mean as top and median as bottom), and inference time for React-OT (blue), one-shot OA-ReactDiff (yellow), and 40-shot OA-ReactDiff with recommender (purple).
    }
    \label{Supp:sumamry}
\end{figure*}

\begin{figure*}[t!]
    \includegraphics[width=0.6\textwidth]{SI/S7_confidence.pdf}
    \caption{\textbf{Mean barrier height of React-OT with different methods for adding confidence data.}
    Yellow corresponds to the confidence model used in the main text.
    Pink corresponds to random selection, giving mean errors oscillating around the overall model performance.
    Orange corresponds to the ideal case, where the lowest error data point is always selected as the data fraction increases.
    }
    \label{Supp:random_confidence}
\end{figure*}

% Ablation studies
% \clearpage
\begin{table*}[th]
\centering 
\caption{\textbf{Statistics of RMSD between xTB and DFT optimized reactants and products.}.
}
\resizebox{0.4\textwidth}{!}{
\begin{tabular}{l|c|cc}\toprule
\multicolumn{1}{c|}{Species} & \multicolumn{1}{c|}{Reaction type} &\multicolumn{2}{c}{RMSD (Å)} \\\midrule
& &mean &median\\\midrule
reactant&uni-molecular&0.070&0.037\\
reactant&multi-molecular&0.084&0.048\\
product&uni-molecular&0.137&0.076\\
product&multi-molecular&0.289&0.204\\
\bottomrule
\end{tabular}}
\label{Supp:table_xtb_rmsd}
\end{table*}

\begin{figure*}[t!]
    \includegraphics[width=0.5\textwidth]{SI/SR1_abs_barrier_vs_barrier_error.pdf}
    \caption{\textbf{Actual vs. React-OT error of barrier height on Transition1x test data.}
    }
    \label{Supp:abs_barrier_vs_barrier_error}
\end{figure*}

\begin{figure*}[t!]
    \includegraphics[width=0.5\textwidth]{SI/SR1_guess_rmsd_vs_rmsd.pdf}
    \caption{\textbf{RMSD of initial guess vs. React-OT generated TS on Transition1x test data.}
    }
    \label{Supp:guess_vs_ot_rmsd}
\end{figure*}

\begin{figure*}[t!]
    \includegraphics[width=0.5\textwidth]{SI/SR1_rmsd_vs_barrier_error.pdf}
    \caption{\textbf{RMSD vs. barrier heigh error for React-OT generated TS on Transition1x test data.}
    }
    \label{Supp:rmsd_vs_barrier_error}
\end{figure*}

\begin{figure*}[t!]
    \includegraphics[width=0.5\textwidth]{SI/multiconf_figure.pdf}
    \caption{\textbf{TS structures generated by React-OT at different reactant and product conformations.}
    React-OT applied on a self-rearrangement reaction at five different conformations, where all reactants (left), TS (middle) and products (right) are shown. For TS, React-OT generated structures are colored with light blue in their C atoms, while the true TS structures are colored with gray in their C atoms. RMSD for each TS conformation is shown in orange.
    }
    \label{Supp:reaction_conformations}
\end{figure*}

% Ablation studies
\begin{table*}[th]
\centering 
\caption{\textbf{Ablation study on React-OT}.
}
\resizebox{0.4\textwidth}{!}{
\begin{tabular}{l|cc}\toprule
\multicolumn{1}{c|}{Model} &\multicolumn{2}{c}{RMSD (Å)} \\\midrule
&mean &median\\\midrule
current&0.1029&0.0527\\
w/o diffusion training&0.1632&0.1202\\
initial TS from normal distribution&0.9860&> 1.0\\
initial TS as reactants&0.1989&0.0962\\
\bottomrule
\end{tabular}}
\label{Supp:table_ablation_study}
\end{table*}

% transferability
\begin{table*}[th]
\centering 
\caption{\textbf{Transferability of React-OT on out-of-distribution datasets}.
}
\resizebox{0.4\textwidth}{!}{
\begin{tabular}{l|cc}\toprule
\multicolumn{1}{c|}{Dataset} &\multicolumn{2}{c}{RMSD (Å)} \\\midrule
&mean &median\\\midrule
Transition1x&0.1029&0.0527\\
Berkholz-15&0.1152&0.0503\\
DielsAlde-41&0.0495&0.0402\\
\bottomrule
\end{tabular}}
\label{Supp:table_ablation_study}
\end{table*}
